# Supplementary material for: Striped twisted state in the orientational epitaxy on quasicrystals
Source: arXiv:2501.06851 source file (2025-01-12)
Supplement: Supplementary file 1 [file SM_novaco.pdf]

# Striped twisted state in the orientational epitaxy on quasicrystals
—
# Supplemental Material

Nicola Manini, Mario Forzanini, Sebastiano Pagano, Marco Bellagente,
Martino Colombo, Dario Bertazioli, and Tommaso Salvalaggio
*Dipartimento di Fisica, Università degli Studi di Milano, Via Celoria 16, 20133 Milano, Italy*

Andrea Vanossi
*CNR-IOM, Consiglio Nazionale delle Ricerche - Istituto Officina dei Materiali,
c/o SISSA Via Bonomea 265, 34136 Trieste, Italy and
International School for Advanced Studies (SISSA), Via Bonomea 265, 34136 Trieste, Italy*

Davide Vanossi
*Department of Chemical and Geological Science, DSCG,
University of Modena and Reggio Emilia, Via Campi 103, 41125 Modena, Italy*

Emanuele Panizon
*The Abdus Salam International Center for Theoretical Physics, Strada Costiera 11, 34151 Trieste, Italy and
Area Science Park, Località Padriciano 99, 34149 Trieste, Italy*

Erio Tosatti and Giuseppe E. Santoro
*International School for Advanced Studies (SISSA), Via Bonomea 265, 34136 Trieste, Italy
The Abdus Salam International Center for Theoretical Physics, Strada Costiera 11, 34151 Trieste, Italy and
CNR-IOM, Consiglio Nazionale delle Ricerche - Istituto Officina dei Materiali,
c/o SISSA Via Bonomea 265, 34136 Trieste, Italy*
(Dated: November 15, 2024)

Supplemental material including mathematical derivations, detail about the numerical implementation, and complementary results relative to a different crystal/quasicrystal spacing ratio.

PACS numbers: 68.35.Af,68.08.De,62.10.+s,62.20.Qp

**Contents**

**S1. Model detail** 2

**S2. A variational formulation of the Novaco-McTague theory for quasicrystals** 3
A. The one-phonon approximation 4
B. Variation of $\theta_{\rm opt}$ with $a_{\rm pot}/a_{\rm coll}$ 6

**S3. The numerical relaxation** 9
A. Finite-size effects 10
B. Weak-coupling range 12
C. Independence of overall translations 12

**S4. The twist-angle dependence for $a_{\rm pot}/a_{\rm coll} = 5.2/5.8$** 15

**References** 15

## S1. MODEL DETAIL

We consider a crystalline harmonic monolayer under the influence of a quasi-crystalline potential. The Hamiltonian can be written as

$$\widehat{H} = \widehat{H}_0 + \widehat{H}_1 = \underbrace{\sum_j \frac{\hat{\mathbf{p}}_j^2}{2M} + \frac{1}{2}\sum_{(jj')} \Phi_{jj'}^{\alpha\alpha'}\, \hat{u}_{j\alpha}\hat{u}_{j'\alpha'}}_{\widehat{H}_0} + \underbrace{\sum_j V(\hat{\mathbf{x}}_j)}_{\widehat{H}_1} . \tag{S.1}$$

Here $\hat{\mathbf{u}}_j$ denotes the displacement of the $j$-th particle from its regular lattice equilibrium position $\mathbf{R}_j$ to $\hat{\mathbf{x}}_j = \mathbf{R}_j + \hat{\mathbf{u}}_j$. Any monoatomic crystal can *a priori* be considered, but in practice we focus on a hexagonal lattice with equilibrium spacing $a_{\rm coll}$ and nearest-neighbor elastic coupling $K$. This setting defines the matrix $\Phi_{jj'}^{\alpha\alpha'}$. $V(\mathbf{x})$ is the potential generated by a rigid periodic or quasi-periodic "substrate" which we take of the following general form involving a finite number of Fourier components:

$$V(\mathbf{x}) = -V_0 \left| \frac{1}{p} \sum_{m=1}^{p} \mathrm{e}^{i\mathbf{k}_m\cdot\mathbf{x}} \right|^2 + \text{constant} = -\frac{V_0}{p^2}\sum_{\mathbf{G}} \mathrm{e}^{-i\mathbf{G}\cdot\mathbf{x}} = -\frac{V_0}{p^2}\sum_{\mathbf{G}} \cos(\mathbf{G}\cdot\mathbf{x}) , \tag{S.2}$$

where

$$\mathbf{k}_m = \frac{c_p \pi}{a_{\rm pot}} \left(\cos\tfrac{2\pi m}{p}, \sin\tfrac{2\pi m}{p}, 0\right) . \tag{S.3}$$

The numerical constants $c_p$ are defined in Table 1 of the Supporting Information of Ref. [1]; in particular $c_3 = \frac{4}{3}$ is relevant for the hexagonal/hexagonal epitaxy, and $c_5 = 2$ is appropriate for the hexagonal/decagonal case. With the $\mathbf{k}_m$ vectors in the "horizontal" surface plane, the energy has no $z$ dependence, so that the dynamics is effectively restricted to two dimensions. Expression (S.2) was used to describe the light pattern resulting from the interference of $p$ identical coherent laser beams incoming from regularly-spaced directions, and with in-plane wavelength $a_{\rm pot}$ [1–9]. Equation (S.2) can also approximately describe the in-plane atomic corrugations that adatoms experience when deposited on top of an atomically flat crystalline/quasicrystalline surface. The set of $\mathbf{G}$'s includes the origin (unimportant, as it yields an overall constant shift to the energy, which we remove in order to keep a null mean value of $V(\mathbf{x})$) and the $p(p-1)$ vectors obtained from:

$$\mathbf{G} = \mathbf{k}_m - \mathbf{k}_{m'} \qquad \text{for } m \neq m' . \tag{S.4}$$

$V(\mathbf{x})$ is normalized in such a way that its range of variation is exactly $V_0$.

The original Novaco-McTague theory [10, 11] considers a crystalline potential, such as the one obtained for $p = 3$ (6 $\mathbf{G}$ vectors) or 4 (twelve $\mathbf{G}$ vectors, with 4 duplicates). The generalization to the quasiperiodic case is realized by taking $p = 5$, that originates twenty $\mathbf{G}$ vectors: the potential $V(\mathbf{x})$ is generated by $\mathbf{k}_m$ forming a regular pentagon, and the $\mathbf{G}$ vectors containing the Fourier components of $V(\mathbf{x})$ form two concentric regular decagons, as illustrated in Fig. 1d of the main text. The sizes of the $\mathbf{G}$ vectors are:

$$|\mathbf{G}_1| = \frac{2\pi}{a_{\rm pot}}\sqrt{\frac{5-\sqrt{5}}{2}} , \quad |\mathbf{G}_2| = \frac{2\pi}{a_{\rm pot}}\sqrt{\frac{5+\sqrt{5}}{2}} . \tag{S.5}$$

The resulting quasiperiodic corrugation potential is illustrated in Fig. 1b of the main text.

The quadratic phonon problem has the standard form. Given the dynamical matrix $\mathbf{D}(\mathbf{q})$ constructed from the elastic couplings $\Phi_{jj'}^{\alpha\alpha'}$, one can calculate eigenvalues and eigenvectors [12]:

$$\mathbf{D}(\mathbf{q}) \cdot \boldsymbol{\epsilon}_{\mathbf{q},s} = M\omega_{\mathbf{q},s}^2 \boldsymbol{\epsilon}_{\mathbf{q},s} . \tag{S.6}$$

The eigenvectors of $\mathbf{D}(\mathbf{q})$ — the polarizations $\boldsymbol{\epsilon}_{\mathbf{q},s}$ of longitudinal and transverse phonons ($s = \mathrm{L}, \mathrm{T}$) — form an orthonormal set [26]:

$$\boldsymbol{\epsilon}_{\mathbf{q},s} \cdot \boldsymbol{\epsilon}_{\mathbf{q},s'} = \delta_{s,s'} . \tag{S.7}$$

A common convention [12] is to choose the phases of the polarizations such that

$$\boldsymbol{\epsilon}_{-\mathbf{q},s} = \boldsymbol{\epsilon}_{\mathbf{q},s} . \tag{S.8}$$

For a finite crystal with $N$ unit cells of lattice vectors $\mathbf{a}_1$ and $\mathbf{a}_2$, with periodic boundary conditions (PBC) in a supercell associated to $N_1\mathbf{a}_1$ and $N_2\mathbf{a}_2$, with $N = N_1N_2$, the wave-vectors $\mathbf{q}$ are exactly $N$ discrete points [12]

$$\mathbf{q} = \frac{n_1}{N_1}\mathbf{b}_1 + \frac{n_2}{N_2}\mathbf{b}_2\,, \tag{S.9}$$

where $\mathbf{b}_1$ and $\mathbf{b}_2$ are the reciprocal lattice basis vectors, $n_1 = 0, \cdots N_1 - 1$ and $n_2 = 0, \cdots N_2 - 1$. The $\mathbf{q}$ vectors can always be taken to belong to the first Brillouin Zone (BZ) [12], by applying a translation by an appropriate reciprocal lattice vector $\boldsymbol{\tau}$. In terms of these quantities, we define the displacements $\hat{\mathbf{u}}_j$ as combinations of phonon creation and destruction operators [12]:

$$\hat{\mathbf{u}}_j = \frac{1}{\sqrt{N}}\sum_{\mathbf{q}}^{\mathrm{BZ}\setminus\mathbf{0}}\sum_s\sqrt{\frac{\hbar}{2M\omega_{\mathbf{q},s}}}\,\mathrm{e}^{i\mathbf{q}\cdot\mathbf{R}_j}\boldsymbol{\epsilon}_{\mathbf{q},s}\left(\hat{a}^\dagger_{-\mathbf{q},s} + \hat{a}_{\mathbf{q},s}\right). \tag{S.10}$$

The corresponding momentum operators are defined in a similar way. $\widehat{H}_0$ is diagonalized in the standard form:

$$\widehat{H}_0 = \sum_{\mathbf{q}}^{\mathrm{BZ}\setminus\mathbf{0}}\sum_s\hbar\omega_{\mathbf{q},s}\left(\hat{a}^\dagger_{\mathbf{q},s}\hat{a}_{\mathbf{q},s} + \frac{1}{2}\right). \tag{S.11}$$

The interaction with the corrugation, Eqs. (S.1) and (S.2), reads:

$$\widehat{H}_1 = -\frac{V_0}{p^2}\sum_j\sum_{\mathbf{G}}\mathrm{e}^{-i\mathbf{G}\cdot\mathbf{R}_j}\mathrm{e}^{-i\mathbf{G}\cdot\hat{\mathbf{u}}_j}\,. \tag{S.12}$$

The dimensionless ratio

$$g = \frac{V_0}{Ka_{\mathrm{coll}}^2} \tag{S.13}$$

is useful to identify the operational regime of the model [13]. When $g \gg 1$, it is energetically very costly for any particle to move away from the the minima of $V(\mathbf{x})$, while it is comparatively cheaper to deform the crystalline arrangement: as a result, the particles tend to remain near the bottom of the corrugation potential wells. On the other hand, the weak-coupling limit $g \ll 1$ sees the corrugation $V(\mathbf{x})$ as a weak perturbation to the harmonic crystal, inducing small deviations from the perfect crystalline arrangement. This weak-coupling perturbative regime is the one addressed by the Novaco-McTague theory [10, 11], that we extend to quasiperiodic potentials.

## S2. A VARIATIONAL FORMULATION OF THE NOVACO-MCTAGUE THEORY FOR QUASICRYSTALS

We now take a variational viewpoint. We assume that the phonons are in a coherent state [14] of the form:

$$|\Psi\rangle = \mathrm{e}^{\sum_{\mathbf{q},s}(z_{\mathbf{q},s}\hat{a}^\dagger_{\mathbf{q},s} - z^*_{\mathbf{q},s}\hat{a}_{\mathbf{q},s})}|0\rangle = \mathrm{e}^{-\frac{1}{2}\sum_{\mathbf{q},s}|z_{\mathbf{q},s}|^2}\mathrm{e}^{\sum_{\mathbf{q},s}z_{\mathbf{q},s}\hat{a}^\dagger_{\mathbf{q},s}}|0\rangle\,, \tag{S.14}$$

where the $z_{\mathbf{q},s}$ are dimensionless variational parameters, with $z_{-\mathbf{q},s} = z^*_{\mathbf{q},s}$. The coherent-state ansatz is consistent with assuming that the effect of $\widehat{H}_1$ is mainly a translation of the equilibrium geometry. We evaluate the average energy of this state, which, dropping the irrelevant zero-point-energy term, reads:

$$E = \langle\Psi|\widehat{H}_0 + \widehat{H}_1|\Psi\rangle = \sum_{\mathbf{q}}^{\mathrm{BZ}\setminus\mathbf{0}}\sum_s\hbar\omega_{\mathbf{q},s}\langle\Psi|\hat{a}^\dagger_{\mathbf{q},s}\hat{a}_{\mathbf{q},s}|\Psi\rangle - \frac{V_0}{p^2}\sum_j\sum_{\mathbf{G}}\mathrm{e}^{-i\mathbf{G}\cdot\mathbf{R}_j}\langle\Psi|\mathrm{e}^{-i\mathbf{G}\cdot\hat{\mathbf{u}}_j}|\Psi\rangle\,. \tag{S.15}$$

Notice that the total energy $E$ is a function of the variational parameters $z_{\mathbf{q},s}$, as well as of the relative displacement of the $\mathbf{R}_j$-lattice with respect to the underlying (fixed) substrate.

The average of the individual terms is fairly simple to calculate on the coherent state, by using the fact that $|\Psi\rangle$ is an eigenstate of the phonon destruction operator [14], $\hat{a}_{\mathbf{q},s}|\Psi\rangle = z_{\mathbf{q},s}|\Psi\rangle$. Hence, for instance:

$$\langle\Psi|\hat{a}^\dagger_{\mathbf{q},s}\hat{a}_{\mathbf{q},s}|\Psi\rangle = |z_{\mathbf{q},s}|^2\,. \tag{S.16}$$

We can calculate the exponential term, $\langle\Psi|\mathrm{e}^{-i\mathbf{G}\cdot\hat{\mathbf{u}}_j}|\Psi\rangle$, after appropriate normal ordering. To do this, let us define $\mathbf{G}\cdot\hat{\mathbf{u}}_j \equiv \hat{A}_j^\dagger + \hat{A}_j$ where $\hat{A}_j$ contains only destruction operators, and $\hat{A}_j^\dagger$ only creation operators:

$$\hat{A}_j = \frac{1}{\sqrt{N}}\sum_{\mathbf{q}}^{\mathrm{BZ}\setminus\mathbf{0}}\sum_s \sqrt{\frac{\hbar}{2M\omega_{\mathbf{q},s}}}\,\mathrm{e}^{i\mathbf{q}\cdot\mathbf{R}_j}\,(\mathbf{G}\cdot\boldsymbol{\epsilon}_{\mathbf{q},s})\,\hat{a}_{\mathbf{q},s}\,. \tag{S.17}$$

The commutator $[\hat{A}_j, \hat{A}_j^\dagger]$ is a c-number which defines a zero-point Debye-Waller [12] factor $W_{\mathbf{G}}$:

$$[\hat{A}_j, \hat{A}_j^\dagger] = \frac{1}{N}\sum_{\mathbf{q}}^{\mathrm{BZ}\setminus\mathbf{0}}\sum_s (\mathbf{G}\cdot\boldsymbol{\epsilon}_{\mathbf{q},s})^2\frac{\hbar}{2M\omega_{\mathbf{q},s}} \equiv 2W_{\mathbf{G}}\,. \tag{S.18}$$

We can therefore use the Baker-Campbell-Hausdorff identity [15]:

$$\mathrm{e}^{-i\mathbf{G}\cdot\hat{\mathbf{u}}_j} = \mathrm{e}^{-i(\hat{A}_j^\dagger+\hat{A}_j)} = \mathrm{e}^{-[\hat{A}_j,\hat{A}_j^\dagger]/2}\mathrm{e}^{-i\hat{A}_j^\dagger}\mathrm{e}^{-i\hat{A}_j} = \mathrm{e}^{-W_{\mathbf{G}}}\mathrm{e}^{-i\hat{A}_j^\dagger}\mathrm{e}^{-i\hat{A}_j} \tag{S.19}$$

which puts the expression in normal-ordered form. The desired average is then:

$$\langle\Psi|\mathrm{e}^{-i\mathbf{G}\cdot\hat{\mathbf{u}}_j}|\Psi\rangle = \mathrm{e}^{-W_{\mathbf{G}}-i\mathbf{G}\cdot\mathbf{u}_j}\,. \tag{S.20}$$

Here $\mathbf{u}_j$ is the average displacement of the $j^{\mathrm{th}}$ particle

$$\mathbf{u}_j = \langle\Psi|\hat{\mathbf{u}}_j|\Psi\rangle = \sum_{\mathbf{q}}^{\mathrm{BZ}\setminus\mathbf{0}}\sum_s\sqrt{\frac{\hbar}{2M\omega_{\mathbf{q},s}}}\left(\mathrm{e}^{i\mathbf{q}\cdot\mathbf{R}_j}\,\boldsymbol{\epsilon}_{\mathbf{q},s}\,\xi_{\mathbf{q},s} + \mathrm{c.c.}\right)\,, \tag{S.21}$$

whose component along $\mathbf{G}$ is given by:

$$\mathbf{G}\cdot\mathbf{u}_j = \sum_{\mathbf{q}}^{\mathrm{BZ}\setminus\mathbf{0}}\sum_s\sqrt{\frac{\hbar}{2M\omega_{\mathbf{q},s}}}\left[\mathrm{e}^{i\mathbf{q}\cdot\mathbf{R}_j}\,(\mathbf{G}\cdot\boldsymbol{\epsilon}_{\mathbf{q},s})\,\xi_{\mathbf{q},s} + \mathrm{c.c.}\right]\,. \tag{S.22}$$

Here $\xi_{\mathbf{q},s} = z_{\mathbf{q},s}/\sqrt{N}$, which turns out to be the correct re-scaling to obtain an extensive total energy. Summarising, the variational total energy per particle is expressed as:

$$\mathcal{E} = \frac{E}{N} = \sum_{\mathbf{q}}^{\mathrm{BZ}\setminus\mathbf{0}}\sum_s\hbar\omega_{\mathbf{q},s}|\xi_{\mathbf{q},s}|^2 - \frac{V_0}{p^2}\sum_{\mathbf{G}}\mathrm{e}^{-W_{\mathbf{G}}}\left(\frac{1}{N}\sum_j\mathrm{e}^{-i\mathbf{G}\cdot\mathbf{R}_j}\mathrm{e}^{-i\mathbf{G}\cdot\mathbf{u}_j}\right)\,. \tag{S.23}$$

This expression should be minimized with respect to the variational parameters $\{\xi_{\mathbf{q},s}\}$. Imposing that $\partial\mathcal{E}/\partial\xi^*_{\mathbf{q},s} = 0$ yields the following nonlinear equation for $\{\xi_{\mathbf{q},s}\}$:

$$\hbar\omega_{\mathbf{q},s}\xi_{\mathbf{q},s} = i\frac{V_0}{p^2}\sqrt{\frac{\hbar}{2M\omega_{\mathbf{q},s}}}\sum_{\mathbf{G}}\mathrm{e}^{-W_{\mathbf{G}}}(\mathbf{G}\cdot\boldsymbol{\epsilon}_{\mathbf{q},s})F_{\mathbf{q},\mathbf{G}}\,, \tag{S.24}$$

where

$$F_{\mathbf{q},\mathbf{G}} = \frac{1}{N}\sum_j\mathrm{e}^{-i(\mathbf{q}-\mathbf{G})\cdot\mathbf{R}_j}\mathrm{e}^{i\mathbf{G}\cdot\mathbf{u}_j}\,. \tag{S.25}$$

depends non-linearly on the $\{\xi_{\mathbf{q},s}\}$ through the term $\mathrm{e}^{i\mathbf{G}\cdot\mathbf{u}_j}$. The zero-point Debye-Waller factor $W_{\mathbf{G}}$ — which is small, in general, for a crystal, unless one considers very small atomic masses — can be evaluated to be entirely negligible (of the order of $10^{-11}$) for the parameters of a colloidal system. We will henceforth neglect it in our equations.

### A. The one-phonon approximation

We now proceed by taking the one-phonon approximation, which will make our variational approach equivalent to that of McTague & Novaco [11] for the crystalline case. The one-phonon approximation consists in truncating the exponential expansion

$$\mathrm{e}^{-i\mathbf{G}\cdot\mathbf{u}_j} \xrightarrow{\text{1-phonon}} 1 - i\mathbf{G}\cdot\mathbf{u}_j \tag{S.26}$$

in Eq. (S.23). At the level of the variational equation (S.24) for the stationary point, it is sufficient to retain only the 0-th order term 1, making $F_{\mathbf{q},\mathbf{G}}$, Eq. (S.25), independent of the variational parameters $\xi_{\mathbf{q},s}$:

$$F_{\mathbf{q},\mathbf{G}} \xrightarrow{\text{1-phonon}} F^{1-\text{ph}}_{\mathbf{q},\mathbf{G}} = \frac{1}{N}\sum_j \mathrm{e}^{-i(\mathbf{q}-\mathbf{G})\cdot\mathbf{R}_j} = \sum_{\boldsymbol{\tau}} \mathrm{e}^{i\boldsymbol{\tau}\cdot\mathbf{R}_0}\delta_{\mathbf{q},\mathbf{G}-\boldsymbol{\tau}}\,. \tag{S.27}$$

$\mathbf{R}_0$ is the position of the central particle in the colloidal lattice, referred to the origin of the quasiperiodic potential. Hence the variational equation (S.24) reads:

$$\hbar\omega_{\mathbf{q},s}\xi_{\mathbf{q},s} \overset{\text{1-ph}}{=} i\frac{V_0}{p^2}\sqrt{\frac{\hbar}{2M\omega_{\mathbf{q},s}}}\sum_{\mathbf{G}}(\mathbf{G}\cdot\boldsymbol{\epsilon}_{\mathbf{q},s})\,F^{1-\text{ph}}_{\mathbf{q},\mathbf{G}} \equiv -g_{\mathbf{q},s}\,, \tag{S.28}$$

where the energies $g_{\mathbf{q},s}$ do not depend on the variational parameters. When considering the total energy per particle, when substituting $\xi_{\mathbf{q},s} = -g_{\mathbf{q},s}/(\hbar\omega_{\mathbf{q},s})$ provided by Eq. (S.28) into Eqs. (S.22) and the 1-phonon approximation of (S.23), one observes that the term with 1 gives a vanishing contribution in the infinite-size limit, because $\sum_j \mathrm{e}^{-i\mathbf{G}\cdot\mathbf{R}_j} = 0$, unless $\mathbf{G}$ accidentally coincides with one of the reciprocal-lattice vectors $\boldsymbol{\tau}$ of the $\mathbf{R}_j$-lattice, which we exclude. Hence:

$$\begin{aligned}\mathcal{E}_{1-\text{ph}} &= \sum_{\mathbf{q}}^{\text{BZ}\setminus\mathbf{0}}\sum_s \hbar\omega_{\mathbf{q},s}|\xi_{\mathbf{q},s}|^2 + i\frac{V_0}{p^2}\sum_{\mathbf{G}}\left(\frac{1}{N}\sum_j \mathrm{e}^{-i\mathbf{G}\cdot\mathbf{R}_j}(\mathbf{G}\cdot\mathbf{u}_j)\right)\\ &= \sum_{\mathbf{q}}^{\text{BZ}\setminus\mathbf{0}}\sum_s \hbar\omega_{\mathbf{q},s}|\xi_{\mathbf{q},s}|^2 + \sum_{\mathbf{q}}^{\text{BZ}\setminus\mathbf{0}}\sum_s\left(g^*_{\mathbf{q},s}\xi_{\mathbf{q},s} + \text{c.c.}\right).\end{aligned} \tag{S.29}$$

By finalizing the substitution of $\xi_{\mathbf{q},s}$ as given by Eq. (S.28) back in the expression (S.29) for $\mathcal{E}_{1-\text{ph}}$ we get:

$$\begin{aligned}\mathcal{E}_{\text{1-ph}} &= -\sum_{s=\text{L,T}}\sum_{\mathbf{q}}^{\text{BZ}\setminus\mathbf{0}}\frac{|g_{\mathbf{q},s}|^2}{\hbar\omega_{\mathbf{q},s}} = -\frac{V_0^2}{2Mp^4}\sum_{s=\text{L,T}}\sum_{\mathbf{q}}^{\text{BZ}\setminus\mathbf{0}}\frac{\left|\sum_{\mathbf{G}}(\mathbf{G}\cdot\boldsymbol{\epsilon}_{\mathbf{q},s})\,\sum_{\boldsymbol{\tau}}\mathrm{e}^{i\boldsymbol{\tau}\cdot\mathbf{R}_0}\delta_{\mathbf{q},\mathbf{G}-\boldsymbol{\tau}}\right|^2}{\omega^2_{\mathbf{q},s}}\\ &= -\frac{V_0^2}{2Mp^4}\sum_{s=\text{L,T}}\sum_{\mathbf{q}}^{\text{BZ}\setminus\mathbf{0}}\sum_{\mathbf{G}}\sum_{\boldsymbol{\tau}}\frac{|\mathbf{G}\cdot\boldsymbol{\epsilon}_{\mathbf{q},s}|^2}{\omega^2_{\mathbf{q},s}}\delta_{\mathbf{q},\mathbf{G}-\boldsymbol{\tau}}\,.\end{aligned} \tag{S.30}$$

Two comments are in order. First: notice the cancellation of the $\hbar$ factors, which tells us that our result captures totally *classical* effects. Second: notice that, in the final step, we have used the fact that the square-modulus of the sum of Kröneker-delta terms does not bring in any cross term, and that $|\mathrm{e}^{i\boldsymbol{\tau}\cdot\mathbf{R}_0}\delta_{\mathbf{q},\mathbf{G}-\boldsymbol{\tau}}|^2 = \delta_{\mathbf{q},\mathbf{G}-\boldsymbol{\tau}}$. As a result no dependence of $\mathcal{E}_{\text{1-ph}}$ on an overall translation $\mathbf{R}_0$ is envisaged. Physically, this result implies the prediction that, as long as the coupling is weak so that the 1-phonon approximation holds, a hexagonal crystal interacting with a decagonal quasiperiodic substrate can slide with *vanishing static friction*, thereby realizing a *superlubric* interface. In Sect. S3 C below we verify numerically that this conclusion holds, up to weak finite-size effects.

The Kröneker-delta terms poses now a problem, since $\mathbf{q}+\boldsymbol{\tau}$ does not generally match any $\mathbf{G}$ for a finite lattice in PBC, where the $\mathbf{q}$'s are discrete, see Eq. (S.9). We therefore take the infinite surface area limit $S_{\text{crystal}} = N\,S_{\text{cell}} \to \infty$ by using the fact that, for any $\mathbf{q}'$,

$$f(\mathbf{q}') = \sum_{\mathbf{q}}^{\text{BZ}} f(\mathbf{q})\delta_{\mathbf{q},\mathbf{q}'} = \frac{(2\pi)^2}{S_{\text{crystal}}}\sum_{\mathbf{q}}^{\text{BZ}} f(\mathbf{q})\;\frac{S_{\text{crystal}}}{(2\pi)^2}\delta_{\mathbf{q},\mathbf{q}'} \overset{N\to\infty}{=} \int_{\text{BZ}}\mathrm{d}\mathbf{q}\,f(\mathbf{q})\,\delta(\mathbf{q}-\mathbf{q}') = f(\mathbf{q}')\,.$$

This leads us to our final expression for the variationally-optimized energy per particle:

$$\mathcal{E}_{\text{1-ph}} \overset{N\to\infty}{=} -\frac{V_0^2}{2Mp^4}\sum_s\sum_{\mathbf{G},\boldsymbol{\tau}}\int_{\text{BZ}}\mathrm{d}\mathbf{q}\frac{|\mathbf{G}\cdot\boldsymbol{\epsilon}_{\mathbf{q},s}|^2}{\omega^2_{\mathbf{q},s}}\delta(\mathbf{q}+\boldsymbol{\tau}-\mathbf{G}) = -\frac{V_0^2}{2Mp^4}\sum_{s=\text{L,T}}\sum_{\mathbf{G}}\sum_{\boldsymbol{\tau}}\left.\frac{|\mathbf{G}\cdot\boldsymbol{\epsilon}_{\mathbf{q},s}|^2}{\omega^2_{\mathbf{q},s}}\right|^{\mathbf{q}\in\text{BZ}}_{\mathbf{q}=\mathbf{G}-\boldsymbol{\tau}}\,. \tag{S.31}$$

Notice that, thanks to the Dirac-delta condition, the sum is restricted to the few $\mathbf{q}$ points satisfying

$$\mathbf{q} = \mathbf{G}-\boldsymbol{\tau}\,. \tag{S.32}$$

For each $\mathbf{G}$, exactly one reciprocal-lattice vector $\boldsymbol{\tau}$ places $\mathbf{q}$ in the first BZ: as a result the number of the matching $\mathbf{q}$'s is the same as the number of $\mathbf{G}$ vectors, namely 20 for the decagonal potential at hand. In this respect, the

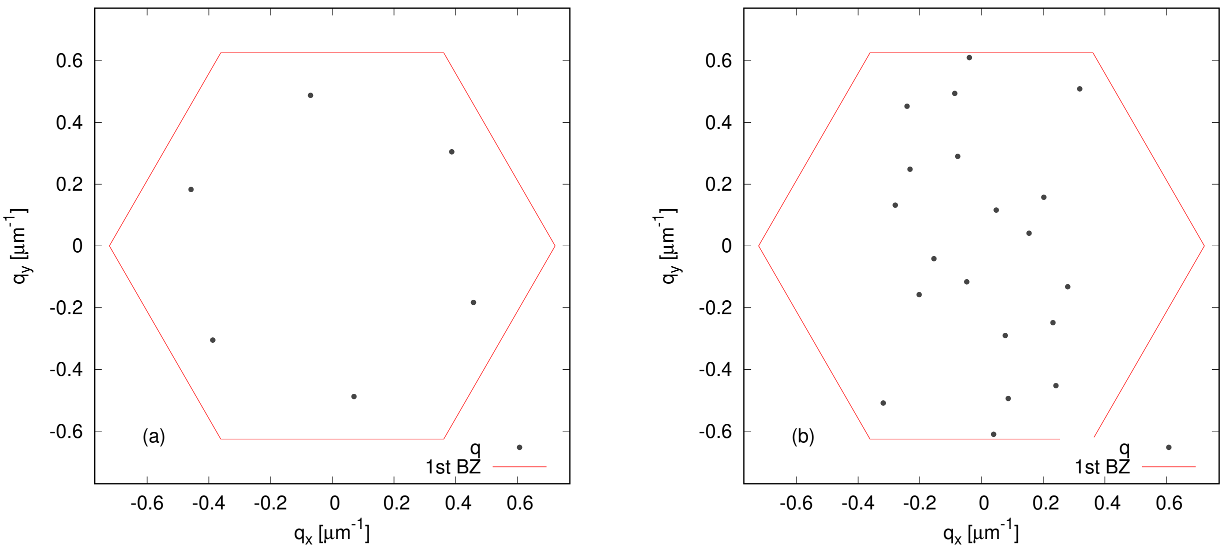


FIG. S1: Red hexagon: the first Brillouin zone of the hexagonal lattice with $a_{\rm coll} = 5.8\,\mu$m. Dots: the $\mathbf{q}$ points obtained by applying Eq. (S.32) to the $p(p-1)$ $\mathbf{G}$ vectors, rotated by $\theta = 2^\circ$, for $a_{\rm pot} = 5.4\,\mu$m. (a) hexagonal potential ($p = 3$); (b) decagonal quasiperiodic potential ($p = 5$), where the $\mathbf{G}$ vectors are those of Fig. 1d.

main difference between the hexagonal-on-hexagonal geometry of Novaco&McTague [10, 11] and the hexagonal-on-decagonal problem at hand is that in the former the $\mathbf{q}$ vectors retain the original hexagonal symmetry see Fig. S1a, while in the latter the only symmetry that the $\mathbf{q}$ vectors retain is the inversions symmetry, i.e. they come in opposite pairs, see Fig. S1b.

To identify the optimal global arrangement, one can further minimize $\mathcal{E}_{\text{1-ph}}$ by tuning the orientation (the "twist angle" $\theta$) of the $\boldsymbol{\tau}$-reciprocal lattice relative to the Fourier $\mathbf{G}$ points of the quasi-crystalline potential. The angular-frequency denominator in Eq. (S.31) tends to favor small-$\mathbf{q}$ *transverse* modes which have a lower sound velocity, and thus smaller $\omega_{\mathbf{q},s}$: the optimal arrangement is obtained for a twist-angle $\theta$ that makes the projections $|\mathbf{G}\cdot\boldsymbol{\epsilon}_{\mathbf{q},s}|$ as large as possible, with the corresponding phonon angular frequencies as small as possible.

Substituting Eq. (S.26) into Eq. (S.21), the average displacement from the initial crystalline position is predicted to be given by:

$$\begin{aligned}\mathbf{u}_j = \langle\Psi|\hat{\mathbf{u}}_j|\Psi\rangle &= \sum_{\mathbf{q}}^{\rm BZ\setminus 0}\sum_s \sqrt{\frac{\hbar}{2M\omega_{\mathbf{q},s}}}\, e^{i\mathbf{q}\cdot\mathbf{R}_j}\,\boldsymbol{\epsilon}_{\mathbf{q},s}\left(\xi^*_{-\mathbf{q},s}+\xi_{\mathbf{q},s}\right)\\ &= -\frac{V_0}{Mp^2}\sum_{s={\rm L,T}}\sum_{\mathbf{G}}\sum_{\boldsymbol{\tau}} \frac{\mathbf{G}\cdot\boldsymbol{\epsilon}_{\mathbf{q},s}}{\omega^2_{\mathbf{q},s}}\boldsymbol{\epsilon}_{\mathbf{q},s}\sin(\mathbf{q}\cdot\mathbf{R}_j)\Big|_{\mathbf{q}=\mathbf{G}-\boldsymbol{\tau}}^{\mathbf{q}\in{\rm BZ}}\,. \end{aligned} \tag{S.33}$$

Given the acoustic phonon behavior at small $|\mathbf{q}|$, the largest distortion will typically be associated to the softest of these phonons, namely the pair of long-wavelength transverse phonons associated to $\mathbf{q} = \pm\mathbf{q}_{\rm min}$, i.e. the pair whose length $|\mathbf{q}|$ is the smallest one.

### B. Variation of $\theta_{\rm opt}$ with $a_{\rm pot}/a_{\rm coll}$

The 1-phonon energy Eq. (S.31) can be evaluated for any given model parameters $a_{\rm pot}$, $a_{\rm coll}$, $V_0$, and twist angle $\theta$ (which sets the mutual rotation of the $\mathbf{G}$ and $\boldsymbol{\tau}$ vectors). In practice the 1-phonon energy depends on the mutual length of these reciprocal vectors defining the crystal/quasicrystal epitaxy, which is uniquely a function of the length ratio $a_{\rm pot}/a_{\rm coll}$. Figure S2 reports examples of angular energetics for three values of $a_{\rm pot}/a_{\rm coll}$. As the energy of Eq. (S.31) scales as $V_0^2$, we report the dimensionless combination $\mathcal{E}_{\text{1-ph}}\,Ka^2_{\rm coll}/V_0^2 = \mathcal{E}_{\text{1-ph}}/(g^2\,Ka^2_{\rm coll})$, which is independent of the coupling strength. This dimensionless factor can be readily converted to whatever coupling one desires, by simply multiplying it by $g^2\,Ka^2_{\rm coll}$. The arrows pointing at the minima in Fig. S2 illustrate that, depending on the length ratio $a_{\rm pot}/a_{\rm coll}$, the optimum twist angle $\theta_{\rm opt}$ can vanish (no twist epitaxy, as in the $a_{\rm pot}/a_{\rm coll} = 0.68$ example), or can be small (e.g. close to $1^\circ$, as for $a_{\rm pot}/a_{\rm coll} = 0.80$), or reach larger values, e.g. $5.3^\circ$ as for $a_{\rm pot}/a_{\rm coll} = 0.93$, namely the ratio investigated in Fig. 3 of the paper.

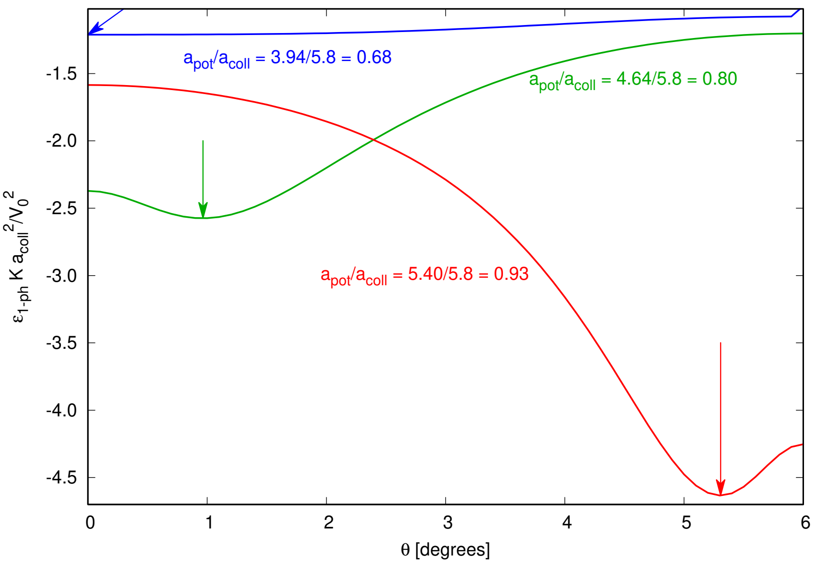


FIG. S2: The 1-phonon energy, Eq. (S.31), as a function of the twist angle $\theta$, for three values of the length ratio $a_{\rm pot}/a_{\rm coll}$. Arrows point at optimal angles $\theta_{\rm opt}$ which minimize this energy.

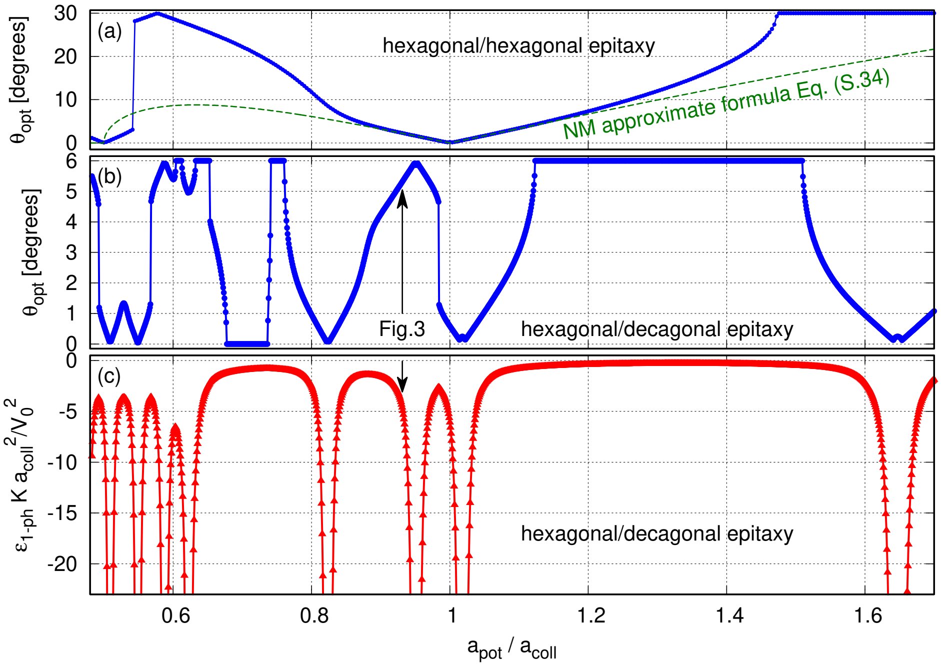


FIG. S3: (a) and (b): the optimum twist angle $\theta_{\rm opt}$ that minimizes the 1-phonon energy, Eq. (S.31), as a function of the ratio $a_{\rm pot}/a_{\rm coll}$ for (a) the traditional hexagonal/hexagonal epitaxy [10] and (b) hexagonal/decagonal geometry (this work). The green dashed curve in (a) reports the approximate Novaco-McTague [11] expression for the optimum angle. The black arrow in (b) points at the specific ratio explored in Fig. 3 of the paper. Panel (c): the 1-phonon energy $\mathcal{E}_{\text{1-ph}}$ at the optimum angle in the hexagonal/decagonal geometry.

For the hexagonal/hexagonal epitaxy McTague&Novaco [11] derive an approximate expression for the optimum twist angle

$$\cos\theta_{\rm opt} = \frac{1+\left(\frac{a_{\rm pot}}{a_{\rm coll}}\right)^2(1+2\eta)}{\frac{a_{\rm pot}}{a_{\rm coll}}\left[2+\eta\left(1+\left(\frac{a_{\rm pot}}{a_{\rm coll}}\right)^2\right)\right]}\,, \qquad \text{where } \eta = \left(\frac{c_{\rm L}}{c_{\rm T}}\right)^2 - 1\,, \tag{S.34}$$

in terms of the longitudinal and transverse speeds of sound $c_{\rm L}$ and $c_{\rm T}$. For the nearest-neighbor hexagonal lattice at hand, $c_{\rm L} = \sqrt{3}\, c_{\rm T}$ so that $\eta = 2$. Figure S3a compares this approximate formula with the exact $\theta_{\rm opt}$ obtained numerically, showing good agreement uniquely in a range near $a_{\rm pot}/a_{\rm coll} \simeq 1$. The commensurate ratios $a_{\rm pot}/a_{\rm coll} = 0.5$ and 1 lead to kink singularities in $\theta_{\rm opt}$. Observe also a jump discontinuity at $a_{\rm pot}/a_{\rm coll} \simeq 0.54$ due to a switch between two competing minima.

The hexagonal/decagonal epitaxy at hand does not lead to a simple analytic expression: we rely on the numerical minimization of Eq. (S.31). Figure S3b shows the resulting optimal twist angle $\theta_{\rm opt}$ as a function of $a_{\rm pot}/a_{\rm coll}$. Observe a rich angular dependence with several plateaus, kinks, and discontinuous jumps: compared to the hexagonal/hexagonal epitaxy where a single ring of $\mathbf{G}$ vectors defines the corrugation potential, in the hexagonal/decagonal geometry at hand, the two rings of $\mathbf{G}$ vectors illustrated in Fig. 1d of the main text lead to more frequent matching conditions as a function of $a_{\rm pot}/a_{\rm coll}$. Figure S3c reports the energy $\mathcal{E}_{\text{1-ph}}$ at the minimum. This energy exhibits negative divergences at specific values of $a_{\rm pot}/a_{\rm coll}$, marked by kinks in panel b. As previously mentioned, these singularities occur at the special geometries for which, at a suitable twist angle, one of the $\mathbf{G}$ vectors generating the quasicrystalline corrugation coincides with one of the reciprocal lattice vectors $\boldsymbol{\tau}$, so that the $\mathbf{q}$ of Eq. (S.32) vanishes. At these special $a_{\rm pot}/a_{\rm coll}$ and $\theta$ points where one such exact commensuration condition holds, the entire theory outlined in Sec. S2 fails: even without any phonon distortion, the overlayer is stabilized by a finite energy proportional to $V_0$.

## S3. THE NUMERICAL RELAXATION

We implemented the classical counterpart of Eq. (S.1) in LAMMPS [16]. Our model consists of a 2D monolayer of point particles individually interacting with the decagonal quasiperiodic potential of Eq. (S.2). For efficiency's sake, the $\mathbf{G}$ vectors involved in the decagonal potential function are pre-calculated once and for all in terms of $\kappa = 2\pi/a_{\rm pot}$:

$$\mathbf{G}_1 = \kappa \left(1 - \cos\frac{2\pi}{5},\, \sin\frac{2\pi}{5}\right) \tag{S.35}$$

$$\mathbf{G}_2 = \kappa \left(1 - \cos\frac{4\pi}{5},\, \sin\frac{4\pi}{5}\right) \tag{S.36}$$

$$\mathbf{G}_3 = \kappa \left(\cos\frac{2\pi}{5} - \cos\frac{4\pi}{5},\, \sin\frac{2\pi}{5} - \sin\frac{4\pi}{5}\right) \tag{S.37}$$

$$\mathbf{G}_4 = \kappa \left(\cos\frac{2\pi}{5} - \cos\frac{4\pi}{5},\, \sin\frac{2\pi}{5} - \sin\frac{6\pi}{5}\right) \tag{S.38}$$

$$\mathbf{G}_5 = \kappa \left(0,\, \sin\frac{2\pi}{5} - \sin\frac{8\pi}{5}\right) \tag{S.39}$$

$$\mathbf{G}_6 = \kappa \left(0,\, \sin\frac{4\pi}{5} - \sin\frac{6\pi}{5}\right) \tag{S.40}$$

All other $\mathbf{G}$ vectors can be trivially expressed in terms of those listed above, so that the calculation of the potential energy, Eq. (S.2), simplifies to

$$\begin{aligned} V(\mathbf{x}) = -\frac{2}{25} V_0 \Big[ &\cos(\mathbf{G}_1\cdot\mathbf{x}) + \cos\big(\overline{\mathbf{G}_1}\cdot\mathbf{x}\big) + \cos(\mathbf{G}_2\cdot\mathbf{x}) + \cos\big(\overline{\mathbf{G}_2}\cdot\mathbf{x}\big) + \cos(\mathbf{G}_3\cdot\mathbf{x}) \\ &+ \cos\big(\overline{\mathbf{G}_3}\cdot\mathbf{x}\big) + \cos(\mathbf{G}_4\cdot\mathbf{x}) + \cos\big(\overline{\mathbf{G}_4}\cdot\mathbf{x}\big) + \cos(\mathbf{G}_5\cdot\mathbf{x}) + \cos(\mathbf{G}_6\cdot\mathbf{x}) \Big], \end{aligned} \tag{S.41}$$

with the notation $\overline{\mathbf{G}} = (G_x, -G_y)$. The resulting force

$$\begin{aligned} \mathbf{F}(\mathbf{x}) &= -\nabla_{\mathbf{x}} V(\mathbf{x}) \\ &= -\frac{2}{25} V_0 \Big[ \mathbf{G}_1 \sin(\mathbf{G}_1\cdot\mathbf{x}) + \overline{\mathbf{G}_1} \sin\big(\overline{\mathbf{G}_1}\cdot\mathbf{x}\big) + \mathbf{G}_2 \sin(\mathbf{G}_2\cdot\mathbf{x}) + \overline{\mathbf{G}_2} \sin\big(\overline{\mathbf{G}_2}\cdot\mathbf{x}\big) + \mathbf{G}_3 \sin(\mathbf{G}_3\cdot\mathbf{x}) \\ &\quad + \overline{\mathbf{G}_3} \sin\big(\overline{\mathbf{G}_3}\cdot\mathbf{x}\big) + \mathbf{G}_4 \sin(\mathbf{G}_4\cdot\mathbf{x}) + \overline{\mathbf{G}_4} \sin\big(\overline{\mathbf{G}_4}\cdot\mathbf{x}\big) + \mathbf{G}_5 \sin(\mathbf{G}_5\cdot\mathbf{x}) + \mathbf{G}_6 \sin(\mathbf{G}_6\cdot\mathbf{x}) \Big]. \end{aligned} \tag{S.42}$$

The particle-particle interaction is modeled by a simple nearest-neighbor harmonic term

$$U_{cc} = \frac{K}{2} \sum_{(i,j)} \left(|\mathbf{r}_i - \mathbf{r}_j| - a_{\rm coll}\right)^2, \tag{S.43}$$

which for small displacements is nearly coincident with its second-order expansion [17]. We adopt the following parameters: nearest-neighbor equilibrium spacing $a_{\rm coll} = 5.8\,\mu\mathrm{m}$, spring constant $K = 0.2\,\mathrm{zJ}\mu\mathrm{m}^{-2}$, and particle mass $M = 31.0593\,\mathrm{pg}$. Pairwise interactions between charged colloidal particles would be described realistically by a screened Coulomb repulsion [1, 3, 4, 9]. However, we adopt the harmonic spring model, in order to prevent the strong anharmonicity of the screened Coulomb interaction to hinder the comparison with the theory based on an harmonic lattice. The adopted parameter values are consistent with the curvature of a realistic screened Coulomb repulsion at the equilibrium spacing $a_{\rm coll}$.

Even though we adopt energy and length scales typical of colloids, we express all energies as a ratio to the natural model energy scale $K a_{\rm coll}^2 = 6.728\,\mathrm{zJ}$, so that the results are readily interpretable even for an atomic overlayer on a crystalline surface.

As for the mutual twist angle $\theta$, the decagonal symmetry of the potential and the symmetries of the hexagonal lattice imply a periodicity of 12°. As a result we can restrict our investigation to the $-6° \le \theta \le 6°$ angular range, which can be further reduced to $0° \le \theta \le 6°$ by noting the angular inversion symmetry $\theta \to -\theta$ of the potential, and therefore of the entire model.

We focus on generic "lattice-incommensurate" situations, namely we adopt values of the length ratio $a_{\rm pot}/a_{\rm coll}$ such that $\mathbf{G} \neq \boldsymbol{\tau}$, hence $\mathbf{q} \neq \mathbf{0}$, for all twist angles $\theta$. In other words, we assume that in reciprocal space the two $\mathbf{G}$-rings with radii given in Eq. (S.5) stay clear from all points $\boldsymbol{\tau}$ of the reciprocal lattice. In concrete, we carry out

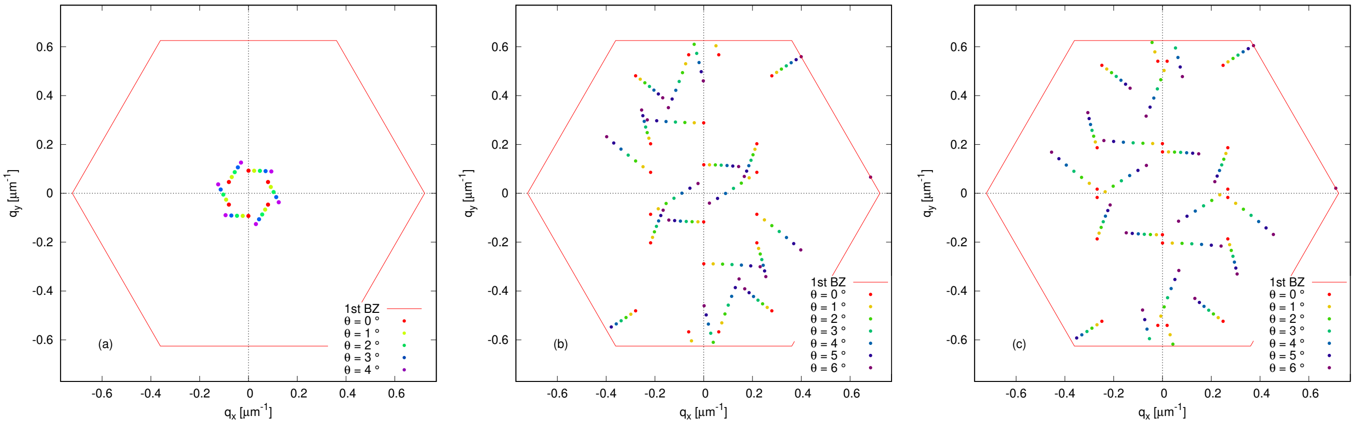


FIG. S4: Red hexagon: the boundary of the first Brillouin zone of the hexagonal lattice with $a_{\rm coll} = 5.8\,\mu$m. Dots: successive locations of the $\mathbf{q}$ points obtained by Eq. (S.32), as the $p(p-1)$ $\mathbf{G}$ vectors of the potential are rotated counterclockwise at the indicated twist angles $\theta$. (a) hexagonal ($p = 3$) potential for $a_{\rm pot} = 5.4\,\mu$m; (b,c) decagonal ($p = 5$) quasiperiodic potential for (b) $a_{\rm pot} = 5.4\,\mu$m or (c) $a_{\rm pot} = 5.2\,\mu$m.

numerical simulations for the following two characteristic lengths of $V(\mathbf{x})$: $a_{\rm pot} = 5.4\,\mu$m, reported in the paper, and $a_{\rm pot} = 5.2\,\mu$m, reported here in Sec. S4.

Figure S1a shows that in hexagonal symmetry, for any $\theta$, the 6 $\mathbf{G}$ vectors generate 6 $\mathbf{q}$ vectors at the vertexes of a regular hexagon inside the 1BZ. In contrast, Fig. S1b shows that in decagonal symmetry the 20 $\mathbf{G}$ vectors drawn in Fig. 1c,d result in irregular patterns of 20 $\mathbf{q}$ vectors. Figure S4 illustrate how the $\mathbf{q}$ vectors evolve as the twist angle $\theta$ is incremented. In the hexagonal/hexagonal epitaxy (Fig. S4a) the 6 $\mathbf{q}$ vectors form a regular hexagon which shrinks near the origin, namely the center of the first 1BZ, as the optimal angle $\theta_{\rm opt}$ is approached. The hexagonal/decagonal geometry differs in the 20 $\mathbf{q}$ vectors forming a nontrivial pattern composed of 10 $(\mathbf{q}, -\mathbf{q})$ pairs, moving as a function of $\theta$. For $a_{\rm pot} = 5.4\,\mu$m Fig. S4b shows that a certain $\mathbf{q}$ pair comes substantially close to $\mathbf{0}$ at some specific twist angle $\simeq 6°$: this geometry is incommensurate, but not too far from matching. Figure S4c indicates that for $a_{\rm pot} = 5.2\,\mu$m at any $\theta$ all $\mathbf{q}$ keep well clear of $\mathbf{0}$: this configuration has a higher degree of mismatch than that of Fig. S4b.

To fix the twist angle $\theta$ in the classical simulations, we cut a circular sample out of a large portion of a hexagonal lattice with spacing $a_{\rm coll}$. We statically fix the positions of the atoms at the edge of the sample at perfect-lattice positions. The total potential energy is therefore a function of the $x$ and $y$ coordinates defining the positions (or, equivalently, the displacements) of all $N$ particles inside this rigid ring. For given values of the twist angle $\theta$, fixed by the external static ring, we utilize LAMMPS to minimize the total potential energy $U$, by relaxing the positions of the $N$ mobile particles inside this fixed static ring.

After testing most minimization algorithms implemented in LAMMPS, we adopt the Fast Inertial Relaxation Engine (FIRE) [18, 19], which proves the most efficient one for the problem at hand. We stick to LAMMPS' default values for most input parameters, except for the time step which we set to 500 ms, best suited to the minimization conditions.

We also tested simulated-annealing minimizations, whose basin-hopping capability could turn out precious for $g \geq 1$ medium-to-strong coupling conditions, where multiple competing minima need to be sorted out. In the present work, however, we focus on the weak-coupling regime $g \ll 1$ where the one-phonon approximation is valid, and where the single minimum adiabatically connected to the perfect-crystal geometry is readily found by FIRE.

For practical purposes, rather than keeping the crystal fixed, and rotating the potential by an angle $\theta$, we proceed the other way around, which is perfectly equivalent. We minimize each twist-angle configuration separately and then collect the total relaxed potential energy $U$ from each angle in order to compare it to the prediction of Eq. (S.31).

### A. Finite-size effects

The theory of Sect. S2 is developed under the assumption of an infinite adsorbed crystalline layer interacting weakly with an infinitely extended potential. Of course our simulations refer to finite samples and finite coupling. Therefore, we need to quantify the effects of finite size and finite coupling on the computed energy.

Due to adopting a zero-average potential $V(\mathbf{x})$, the corrugation energy at randomly placed points vanishes on average. Since the points in the perfect crystal are unrelated to the quasicrystalline potential, they can be seen as random sampling of the latter. Therefore the potential energy per particle of a rigid (unrelaxed) crystal should vanish in the infinite-size limit, but it deviates from 0 in any finite sample. Figure S5 reports precisely this potential-energy

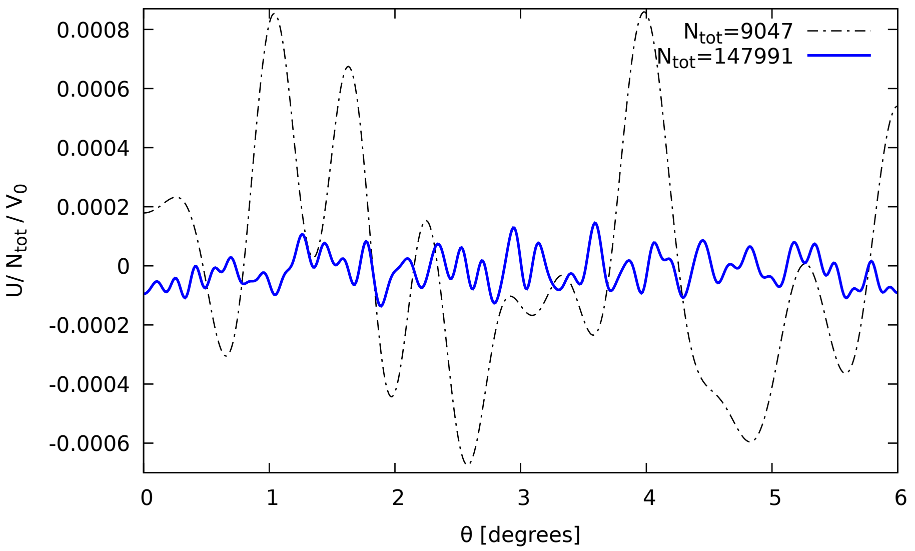


FIG. S5: Edge effects: comparison of the potential energy per particle of two rigid (non relaxed) circular samples of different sizes, as a function of the twist angle $\theta$ of the lattice relative to the underlying decagonal quasicrystalline potential, for $a_{\rm coll} = 5.8\,\mu$m, $a_{\rm pot} = 5.2\,\mu$m, $V_0 = 0.00148\,K a_{\rm coll}^2$.

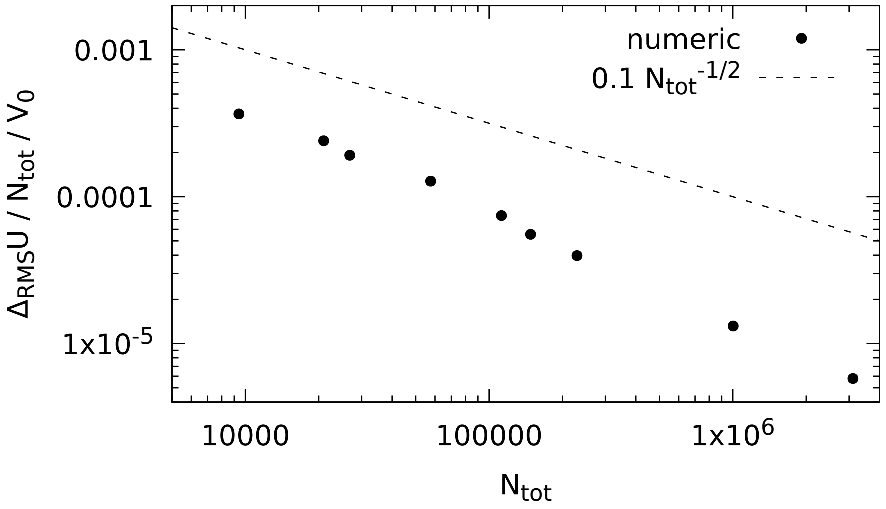


FIG. S6: Edge effects: size dependence of the amplitude of edge-related angular energy fluctuations (see Fig. S5) of a rigid circular sample, evaluated as the root mean square (RMS) deviation of $U(\theta)$. As indicated by the fit, these RMS fluctuations decrease with increasing size faster than $N_{\rm tot}^{-1/2}$.

deviation as a function of the twist angle $\theta$ for circular samples of two sizes. As expected, this energy fluctuates around 0, and its fluctuations decrease in amplitude and increase in frequency as the sample size increases.

The finite-size effects on $U$ should be of the order of the number of particles perturbed by the sample edge. For a circular sample consisting of $N_{\rm tot}$ particles, this is of the order of $N_{\rm tot}^{1/2}$ particles: as a result, the fluctuations on $U/N_{\rm tot}$ should decrease at least as $N_{\rm tot}^{-1/2}$. Figure S6 indeed shows that for our circular samples the per-particle RMS amplitude of the energy fluctuations decreases with size faster than $N_{\rm tot}^{-1/2}$.

These finite-size effects are quite small. In order to further mitigate them in the numerical results, rather than the absolute potential energy $U$, we report the difference $\Delta U$ between the initial unrelaxed energy (namely the energy of the rigid crystal, e.g. the one reported in Fig. S5) and the final relaxed energy for the same angle.

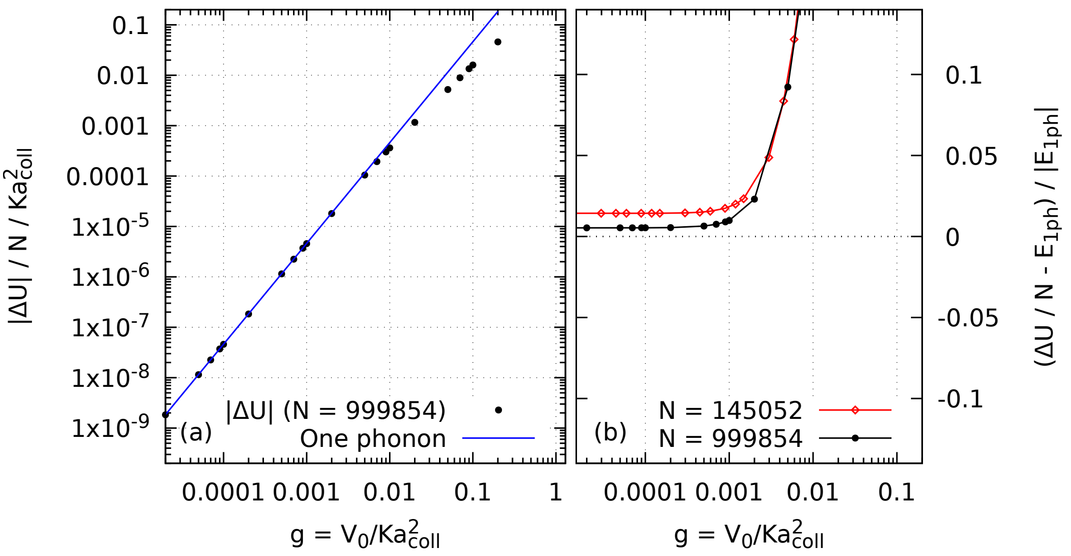


FIG. S7: Validity limit of the weak-coupling range. (a) The absolute value of the relaxation energy per particle $\Delta U/N$ (points) compared with the weak-coupling one-phonon approximation (line), as a function of the corrugation potential amplitude $V_0$, expressed as a dimensionless ratio $g$. (b) Relative deviation between the simulation results and the one-phonon approximation, showing visible variations above $g > 2 \times 10^{-4}$. Residual deviations for $g \to 0$ are finite-size effects. Calculations are carried out at the twist angle $\theta = 5.2°$, $a_{\rm pot}/a_{\rm coll} = 5.4\,\mu{\rm m}/(5.8\,\mu{\rm m})$, for two sizes: $N = 145052$ ($N_{\rm tot} = 147991$), and $N = 999854$, ($N_{\rm tot} = 1003633$).

### B. Weak-coupling range

Beside finite-size effects, we must determine the range of amplitude $V_0$ for which the corrugation can rightfully be considered small when compared to the adsorbed layer's elastic energy, i.e. the $g \ll 1$ weak-coupling expansion is appropriate. In the small-corrugation regime the energy lowering is predicted to be quadratic in the potential amplitude $V_0$, see Eq. (S.31).

To verify where this quadratic dependence holds, at fixed $\theta$ we evaluate the potential-energy lowering $|\Delta U|$ for several values of the potential amplitude $V_0$. Figures S7 and S8 show that deviations from the one-phonon quadratic prediction become essentially negligible for $g = V_0/(K a_{\rm coll}^2) \leq 10^{-4}$.

### C. Independence of overall translations

As discussed in Sect. S2 A, the energy is expected to be entirely independent of an overall translation $\mathbf{R}_0$. We verify this point numerically by evaluating the relaxation energy $\Delta U$ as a function of an overall displacement $\mathbf{R}_0$ of the circular sample. In Fig. S9 we consider the $\theta = \theta_{\rm opt}$ twist angle for the $a_{\rm pot}/a_{\rm coll} = 5.4\,\mu{\rm m}/(5.8\,\mu{\rm m})$ interface, and carry out translations in the direction of the shortest $\mathbf{q}$ vector and perpendicular to it. The small nonperiodic fluctuations of the energy decrease visibly with increasing sample size. Figure S10 shows that the RMS amplitude of these energy fluctuations decreases with size faster than $N_{\rm tot}^{-1/2}$, thereby confirming the superlubric nature of this interface [20–25].

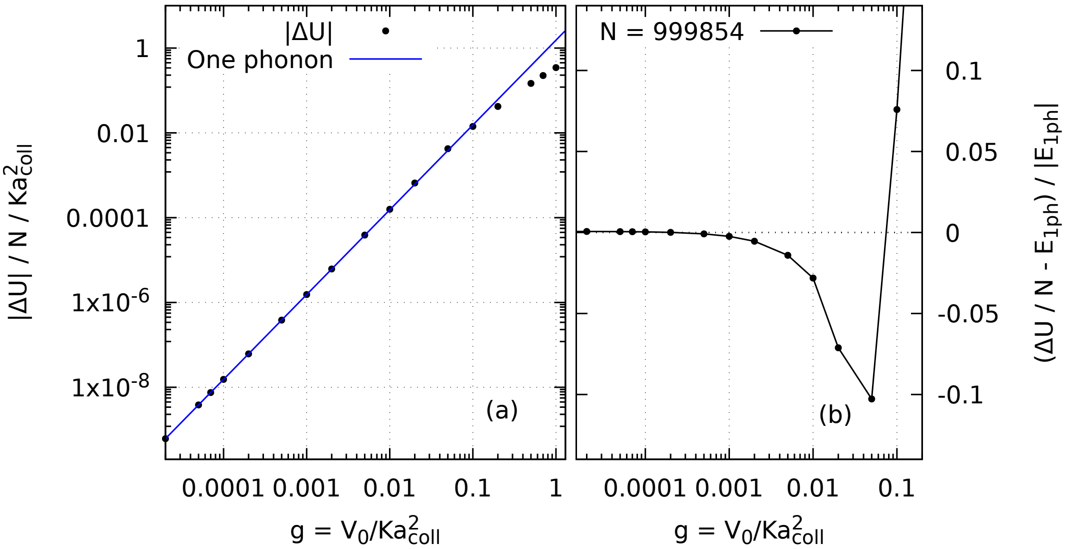


FIG. S8: Same as Fig. S7, but for $a_{\rm pot}/a_{\rm coll} = 5.2\,\mu{\rm m}/5.8\,\mu{\rm m}$, and at the twist angle $\theta = 4.1^\circ$.

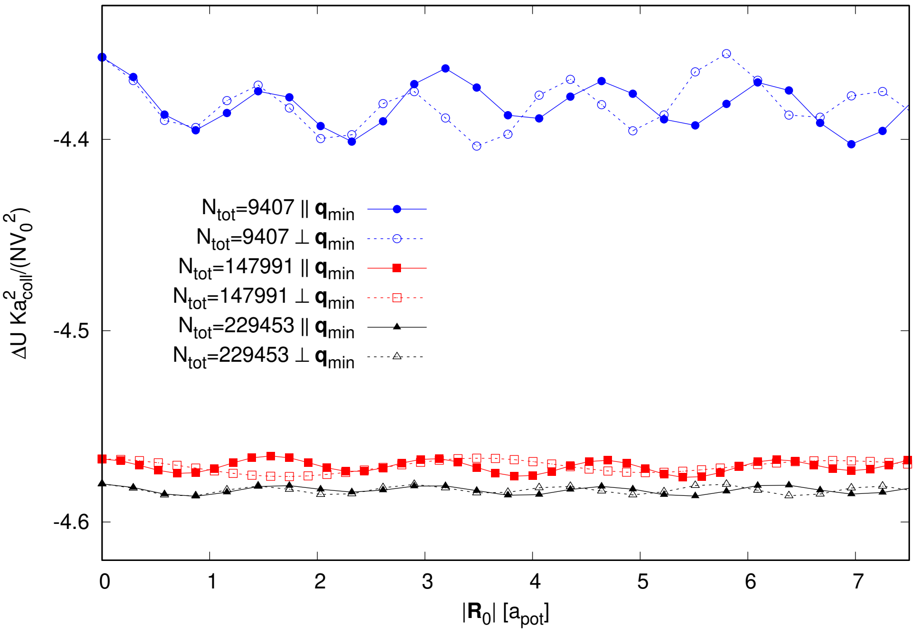


FIG. S9: Effect of the translation of the sample center $\mathbf{R}_0$ on the numerically relaxed energy per particle. The decrease in amplitude of the quasiperiodic energy fluctuations for increasing size $N_{\rm tot}$ suggests that these fluctuations are an effect of the boundary and would vanish for an infinite-size contact. Translations are carried out with $\mathbf{R}_0$ along the shortest $\mathbf{q}$ vector (solid lines) and perpendicularly to it (dashed lines). The simulation parameters are the following: mismatch ratio $a_{\rm pot}/a_{\rm coll} = 5.4\,\mu{\rm m}/(5.8\,\mu{\rm m})$, twist angle $\theta = \theta_{\rm opt} \simeq 5.3^\circ$ and $g = 10^{-4}$.

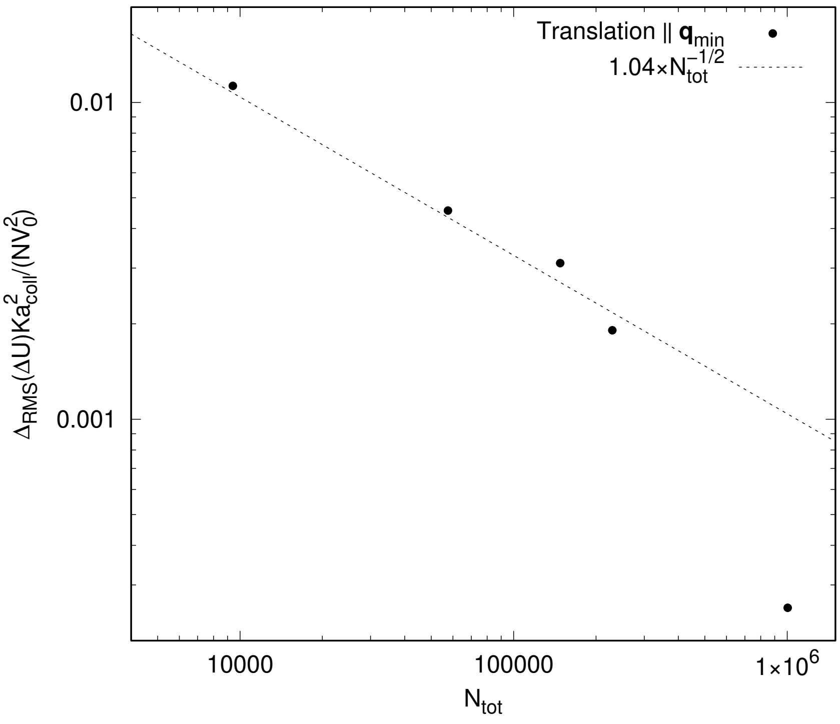


FIG. S10: Size dependence of the amplitude of the edge-related relaxed energy fluctuations as a function of the position $\mathbf{R}_0$ of the center of the sample as is translated in the direction $\mathbf{q}_{\mathrm{min}}$ vector (solid lines of Fig. S9). The fluctuations are evaluated as the RMS deviation of the relaxation energy $\Delta U(\mathbf{R}_0)$ shown in Fig. S9, where $\mathbf{R}_0$ is the overall translation.

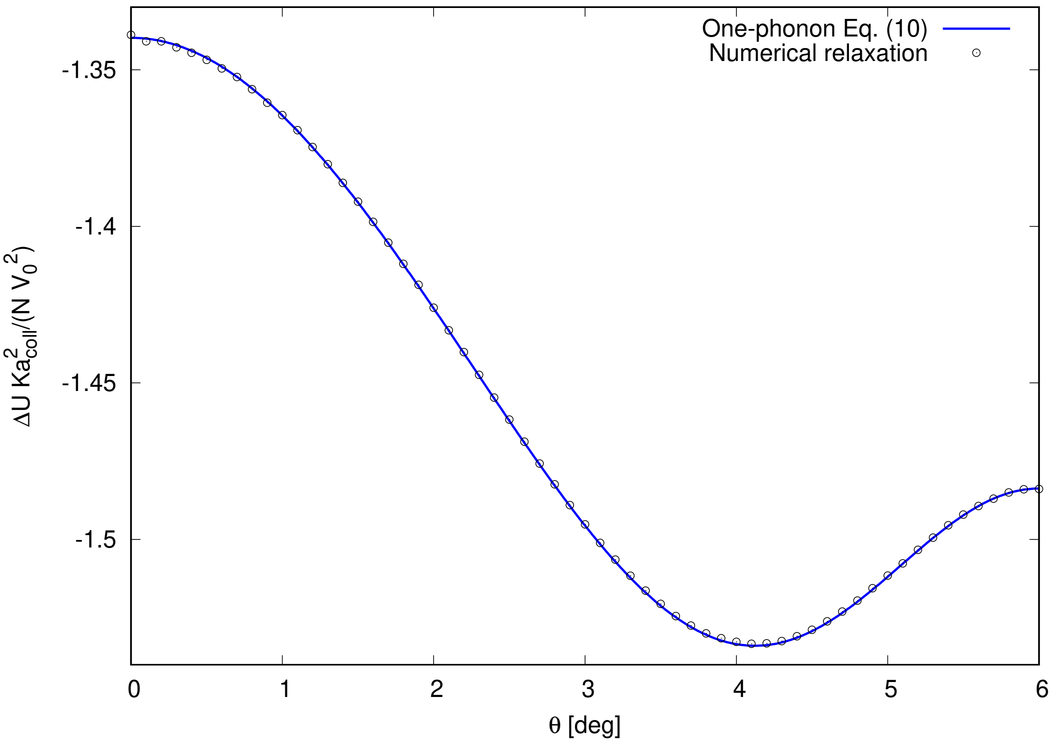


FIG. S11: Comparison of the numerically relaxed total potential energy per particle as a function of the twist angle $\theta$ (points), with the one-phonon result of the theory Eq. (S.31) (line), for a mismatch ratio $a_{\rm pot}/a_{\rm coll} = 5.2\,\mu{\rm m}/(5.8\,\mu{\rm m})$ different from the one reported in Fig. 3 of the main text. Numerical relaxation are carried out for $V_0 = 10^{-4}\,Ka^2_{\rm coll}$, and $N = 999854$.

## S4. THE TWIST-ANGLE DEPENDENCE FOR $a_{\rm pot}/a_{\rm coll} = 5.2/5.8$

We compare the energy lowering per particle $\Delta U/N$ obtained by numerical relaxation of a circular sample of $N = 999854$ particles ($N_{\rm tot} = 1003633$) with the one-phonon expression Eq. (S.31). In the paper these quantities are evaluated as a function of the twist angle $\theta$ and reported in Fig. 3 for the ratio $a_{\rm pot}/a_{\rm coll} = 5.4\,\mu{\rm m}/(5.8\,\mu{\rm m})$. A similar calculation is reported here in Fig. S11 for a different ratio $a_{\rm pot}/a_{\rm coll} = 5.2\,\mu{\rm m}/(5.8\,\mu{\rm m})$. As illustrated in Fig. S4, this second ratio remains farther away from matching for all $\theta$. For both ratios, the numerical minimizations show a good quantitative agreement with the one-phonon theory, without any fitting parameter.

Comparing Fig. 3 with Fig. S11, we see that the less-mismatched geometry $a_{\rm pot}/a_{\rm coll} = 5.4\,\mu{\rm m}/(5.8\,\mu{\rm m})$ leads to a prominent optimal angular minimum, at $\theta_{\rm opt} \simeq 5.31^\circ$, because of the smaller $|\omega_{\mathbf{q},s}|^2$ at the denominator of Eq. (S.31), due to the closeness of $\mathbf{q}$ to $\mathbf{0}$ at the optimal angle, illustrated in Fig. S4b,c. On the other hand, the more mismatched geometry $a_{\rm pot}/a_{\rm coll} = 5.2\,\mu{\rm m}/(5.8\,\mu{\rm m})$ of Fig. S11 leads to a smaller energy lowering for all angles, and to a shallower minimum at the optimal angle $\theta_{\rm opt} \simeq 4.12^\circ$.

[1] A. Vanossi, N. Manini, and E. Tosatti, Proc. Natl. Acad. Sci. USA **109**, 16429 (2012).
[2] T. Brazda, A. Silva, N. Manini, A. Vanossi, R. Guerra, E. Tosatti, and C. Bechinger, Phys. Rev. X **8**, 011050 (2018).
[3] J. Mikhael, G. Gera, T. Bohlein, and C. Bechinger, Soft Matter **7**, 1352 (2011).
[4] T. Bohlein, J. Mikhael, and C. Bechinger, Nat. Mater. **11**, 126 (2012).
[5] T. Bohlein and C. Bechinger, Phys. Rev. Lett. **109**, 058301 (2012).
[6] M. Brunner, C. Bechinger, W. Strepp, V. Lobaskin, and H. H. von Grunberg, Europhys. Lett. **58**, 926 (2002).
[7] K. Mangold, P. Leiderer, and C. Bechinger, Phys. Rev. Lett. **90**, 158302 (2003).
[8] S. Bleil, H. H. von Grünberg, J. Dobnikar, R. C. neda Priego, and C. Bechinger, Europhys. Lett. **73**, 450 (2006).
[9] J. Mikhael, M. Schmiedeberg, S. Rausch, J. Roth, H. Stark, and C. Bechinger, Proc. Natl. Acad. Sci. U.S.A. **107**, 7214 (2010).
[10] A. D. Novaco and J. P. McTague, Phys. Rev. Lett. **38**, 1286 (1977).

[11] J. P. McTague and A. D. Novaco, Phys. Rev. B **19**, 5299 (1979).
[12] N. Ashcroft and M. Mermin, *Solid State Physics* (Holt-Saunders, Philadelphia, 1976).
[13] L. Floría and J. Mazo, Adv. Phys. **45**, 505 (1996).
[14] G. Mahan, *Many-Particles Physics* (Plenum, New York, 1981).
[15] R. M. Wilcox, J. Math. Phys. **8**, 962 (1967).
[16] S. Plimpton, J. Comput. Phys. **117**, 1 (1995).
[17] J. Norell, A. Fasolino, and A. S. de Wijn, Phys. Rev. E **94**, 023001 (2016).
[18] E. Bitzek, P. Koskinen, F. Gähler, M. Moseler, and P. Gumbsch, Phys. Rev. Lett. **97**, 170201 (2006).
[19] J. Guénolé, W. G. Nöhring, A. Vaid, F. Houllé, Z. Xie, A. Prakash, and E. Bitzek, Comp. Mat. Sci. **175**, 109584 (2020).
[20] O. M. Braun, N. Manini, and E. Tosatti, Phys. Rev. Lett. **110**, 085503 (2013).
[21] N. Varini, A. Vanossi, R. Guerra, D. Mandelli, R. Capozza, and E. Tosatti, Nanoscale **7**, 2093 (2015).
[22] E. Koren and U. Duerig, Phys. Rev. B **94**, 045401 (2016).
[23] J. Wang, W. Cao, Y. Song, C. Qu, Q. Zheng, and M. Ma, Nano Lett. **19**, 7735 (2019).
[24] W. Yan, X. Gao, W. Ouyang, Z. Liu, O. Hod, and M. Urbakh, J. Mech. Phys. Solids **185**, 105555 (2024).
[25] J. Wang, A. Khosravi, A. Vanossi, and E. Tosatti, Rev. Mod. Phys. **96**, 011002 (2024).
[26] For a monoatomic crystal [12], the matrix $\mathbf{D}(\mathbf{q})$ is real for any $\mathbf{q}$: consequently, the polarization eigenvectors $\boldsymbol{\epsilon}_{\mathbf{q},s}$ can also be taken real.
